# Supplementary material for: A Graph is Worth $K$ Words: Euclideanizing Graph using Pure Transformer
Source: arXiv:2402.02464 source file (2024-05-29)
Supplement: Supplementary file 1 [file graphsgpt_appendix.pdf]

## A. Representation

For property prediction, we present additional baseline results in Table 5. When applying graph mixup, the training samples are drawn from the original data with probability  $p_{self}$  and from mixed data with probability  $(1 - p_{self})$ . The mixup hyperparameter  $\alpha$  and  $p_{self}$  are shown in Table 6.

Table 5: Results of molecular property prediction. We report the mean (standard deviation) metrics of 10 runs with standard scaffold splitting (not random scaffold splitting). The **best** results and the second best are highlighted.

|             |                                  | ROC-AUC $\uparrow$ |                   |                   |                   |                   |                   | RMSD $\downarrow$    |                      |                      |
|-------------|----------------------------------|--------------------|-------------------|-------------------|-------------------|-------------------|-------------------|----------------------|----------------------|----------------------|
|             |                                  | Tox21              | ToxCast           | Sider             | HIV               | BBBP              | Bace              | ESOL                 | FreeSolv             | Lipo                 |
| # Molecules |                                  | 7,831              | 8,575             | 1,427             | 41,127            | 2,039             | 1,513             | 1128                 | 642                  | 4200                 |
| # Tasks     |                                  | 12                 | 617               | 27                | 1                 | 1                 | 1                 | 1                    | 1                    | 1                    |
| No pretrain | GINs                             | 74.6 (0.4)         | 61.7 (0.5)        | 58.2 (1.7)        | 75.5 (0.8)        | 65.7 (3.3)        | 72.4 (3.8)        | 1.050 (0.008)        | 2.082 (0.082)        | 0.683 (0.016)        |
|             | Graph2Seq-1W                     | 74.0 (0.4)         | 62.6 (0.3)        | 66.6 (1.1)        | 73.6 (3.4)        | 68.3 (1.4)        | 77.3 (1.2)        | 0.953 (0.025)        | 1.936 (0.246)        | 0.907 (0.021)        |
|             | Relative gain to GIN             | -0.8%              | +1.4%             | +12.6%            | -2.6%             | +3.8%             | +6.3%             | +10.2%               | +7.5%                | -24.7%               |
| Pretrain    | InfoGraph (Sun et al., 2019)     | 73.3 (0.6)         | 61.8 (0.4)        | 58.7 (0.6)        | 75.4 (4.3)        | 68.7 (0.6)        | 74.3 (2.6)        |                      |                      |                      |
|             | GPT-GNN (Hu et al., 2020b)       | 74.9 (0.3)         | 62.5 (0.4)        | 58.1 (0.3)        | 58.3 (5.2)        | 64.5 (1.4)        | 77.9 (3.2)        |                      |                      |                      |
|             | EdgePred (Hamilton et al., 2017) | 76.0 (0.6)         | 64.1 (0.6)        | 60.4 (0.7)        | 64.1 (3.7)        | 67.3 (2.4)        | 77.3 (3.5)        |                      |                      |                      |
|             | ContextPred (Hu et al., 2019)    | 73.6 (0.3)         | 62.6 (0.6)        | 59.7 (1.8)        | 74.0 (3.4)        | 70.6 (1.5)        | 78.8 (1.2)        |                      |                      |                      |
|             | GraphLoG (Xu et al., 2021)       | 75.0 (0.6)         | 63.4 (0.6)        | 59.6 (1.9)        | 75.7 (2.4)        | 68.7 (1.6)        | 78.6 (1.0)        |                      |                      |                      |
|             | G-Contextual (Rong et al., 2020) | 75.0 (0.6)         | 62.8 (0.7)        | 58.7 (1.0)        | 60.6 (5.2)        | 69.9 (2.1)        | 79.3 (1.1)        |                      |                      |                      |
|             | G-Motif (Rong et al., 2020)      | 73.6 (0.7)         | 62.3 (0.6)        | 61.0 (1.5)        | 77.7 (2.7)        | 66.9 (3.1)        | 73.0 (3.3)        |                      |                      |                      |
|             | AD-GCL (Suresh et al., 2021)     | 74.9 (0.4)         | 63.4 (0.7)        | 61.5 (0.9)        | 77.2 (2.7)        | 70.7 (0.3)        | 76.6 (1.5)        |                      |                      |                      |
|             | JOAO (You et al., 2021)          | 74.8 (0.6)         | 62.8 (0.7)        | 60.4 (1.5)        | 66.6 (3.1)        | 66.4 (1.0)        | 73.2 (1.6)        | 1.120 (0.003)        |                      | 0.708 (0.004)        |
|             | SimGRACE (Xia et al., 2022a)     | 74.4 (0.3)         | 62.6 (0.7)        | 60.2 (0.9)        | 75.5 (2.0)        | 71.2 (1.1)        | 74.9 (2.0)        |                      |                      |                      |
|             | GraphCL (You et al., 2020)       | 75.1 (0.7)         | 63.0 (0.4)        | 59.8 (1.3)        | 77.5 (3.8)        | 67.8 (2.4)        | 74.6 (2.1)        | 0.947 (0.038)        | 2.233 (0.261)        | 0.739 (0.009)        |
|             | GraphMAE (Hou et al., 2022)      | 75.2 (0.9)         | 63.6 (0.3)        | 60.5 (1.2)        | 76.5 (3.0)        | 71.2 (1.0)        | 78.2 (1.5)        |                      |                      |                      |
|             | 3D InfoMax (Stärk et al., 2022)  | 74.5 (0.7)         | 63.5 (0.8)        | 56.8 (2.1)        | 62.7 (3.3)        | 69.1 (1.2)        | 78.6 (1.9)        | <u>0.894</u> (0.028) | 2.337 (0.227)        | 0.695 (0.012)        |
|             | GraphMVP (Liu et al., 2021a)     | 74.9 (0.8)         | 63.1 (0.2)        | 60.2 (1.1)        | <u>79.1</u> (2.8) | 70.8 (0.5)        | 79.3 (1.5)        | 1.029 (0.033)        |                      | <u>0.681</u> (0.010) |
|             | MGSSL (Zhang et al., 2021)       | 75.2 (0.6)         | 63.3 (0.5)        | 61.6 (1.0)        | 77.1 (4.5)        | 68.8 (0.6)        | 78.8 (0.9)        |                      |                      |                      |
|             | AttrMask (Hu et al., 2019)       | 75.1 (0.9)         | 63.3 (0.6)        | 60.5 (0.9)        | 73.5 (4.3)        | 65.2 (1.4)        | 77.8 (1.8)        | 1.100 (0.006)        | 2.764 (0.002)        | 0.739 (0.003)        |
|             | MolCLR (Wang et al., 2022)       | 75.0 (0.2)         |                   | 58.9 (1.4)        | 78.1 (0.5)        | <u>72.2</u> (2.1) | 82.4 (0.9)        | 1.271 (0.040)        | 2.594 (0.249)        | 0.691 (0.004)        |
|             | Graphformer (Rong et al., 2020)  | 74.3 (0.1)         | <b>65.4</b> (0.4) | <u>64.8</u> (0.6) | 62.5 (0.9)        | 70.0 (0.1)        | <u>82.6</u> (0.7) | 0.983 (0.090)        | <u>2.176</u> (0.052) | 0.817 (0.008)        |
|             | Mole-BERT (Xia et al., 2023)     | <u>76.8</u> (0.5)  | <u>64.3</u> (0.2) | 62.8 (1.1)        | 78.9 (3.0)        | 71.9 (1.6)        | 80.8 (1.4)        | 1.015 (0.030)        |                      | <b>0.676</b> (0.017) |
|             | Relative gain to GIN             | +2.9%              | +6.0%             | +11.3%            | +4.8%             | +9.9%             | +14.1%            | +14.9%               | -4.5%                | +1.0%                |
| Pretrain    | Graph2Seq-1W                     | <b>76.9</b> (0.3)  | <b>65.4</b> (0.5) | <b>68.2</b> (0.9) | <b>79.4</b> (3.9) | <b>72.8</b> (1.5) | <b>83.4</b> (1.0) | <b>0.860</b> (0.024) | <b>1.797</b> (0.237) | 0.716 (0.019)        |
|             | Relative gain to GIN             | +3.1%              | +6.0%             | +17.2%            | +5.2%             | +10.8%            | +15.2%            | +18.1%               | +13.7%               | -4.8%                |
|             | Relative gain to Graph2Seq-1W    | +3.9%              | +4.5%             | +2.4%             | +7.9%             | +6.6%             | +7.9%             | +9.8%                | +7.2%                | +21.1%               |

|                      | Tox21 | ToxCast | Sider | HIV  | BBBP       | BACE | ESOL | FreeSolv | LIPO |
|----------------------|-------|---------|-------|------|------------|------|------|----------|------|
| batch size           | 16    | 16      | 16    | 64   | 128        | 16   | 16   | 64       | 16   |
| lr                   | 1e-5  | 5e-5    | 1e-4  | 1e-4 | 5e-4       | 1e-5 | 1e-4 | 1e-4     | 5e-5 |
| dropout              | 0.0   | 0.0     | 0.0   | 0.0  | 0.1 or 0.3 | 0.0  | 0.1  | 0.1      | 0.0  |
| epoch                | 50    | 50      | 50    | 50   | 50 or 100  | 50   | 50   | 50       | 50   |
| $\alpha$ for mixup   | 0.5   | 0.1     | 0.5   | 0.5  | 0.5        | 0.5  | 0.5  | 0.5      | 0.1  |
| $p_{self}$ for mixup | 0.7   | 0.7     | 0.7   | 0.5  | 0.5        | 0.7  | 0.7  | 0.9      | 0.7  |

Table 6: Hyperparameters for property prediction.

## B. Generation

### B.1. Unconditional Generation

We introduce metrics (Bagal et al., 2021) of unconditional generation as follows:

- **Validity:** the fraction of a generated molecules that are valid. We use RDkit for validity check of molecules. Validity measures how well the model has learned the SMILES grammar and the valency of atoms.
- **Uniqueness:** the fraction of valid generated molecules that are unique. Low uniqueness highlights repetitive molecule generation and a low level of distribution learning by the model.
- **Novelty:** the fraction of valid unique generated molecules that are not in the training set. Low novelty is a sign of overfitting. We do not want the model to memorize the training data.
- **Internal Diversity (IntDiv<sub>p</sub>):** measures the diversity of the generated molecules, which is a metric specially designed to check for mode collapse or whether the model keeps generating similar structures. This uses the power ( $p$ ) mean of the Tanimoto similarity ( $T$ ) between the fingerprints of all pairs of molecules ( $s1, s2$ ) in the generated set ( $S$ ).

$$\text{InvDiv}_p(S) = 1 - \sqrt[p]{\frac{1}{|S|^2} \sum_{s1, s2 \in S} T(s1, s2)^p} \quad (14)$$

### B.2. Conditional Generation

In this section, we provide a detailed description of the conditions used for conditional generation:

- **QED (Quantitative Estimate of Drug-likeness)** is a measure that quantifies the “drug-likeness” of a molecule based on its pharmacokinetic profile, ranging from 0 to 1.
- **SA (Synthetic Accessibility)** is a score that predicts the difficulty of synthesizing a molecule based on multiple factors. Lower SA scores indicate easier synthesis.
- **logP (Partition Coefficient)** is a key parameter in studies of drug absorption and distribution in the body that measuring a molecule’s hydrophobicity.
- **Scaffold** is the core structure of a molecule, which typically includes rings and the atoms that connect them. It provides a framework upon which different functional groups can be added to create new molecules.

In order to integrate conditional information into our model, we set aside an additional 100M from the Zinc15 database (Irwin & Shoichet, 2005) for fine-tuning, which we denote as the dataset  $\mathcal{D}_{\mathcal{G}}$ . For each molecule  $\mathcal{G} \in \mathcal{D}_{\mathcal{G}}$ , we compute its property values  $v_{\text{QED}}$ ,  $v_{\text{SA}}$  and  $v_{\text{logP}}$ , and normalize these values based on those in  $\mathcal{D}_{\mathcal{G}}$ , yielding  $\bar{v}_{\text{QED}}$ ,  $\bar{v}_{\text{SA}}$  and  $\bar{v}_{\text{logP}}$ .

The Graph2Seq model takes all properties and scaffolds as input and transforms them into the graph word sequence  $\mathcal{W} = [w_1, w_2, \dots, w_k]$ , which is subsequently decoded by GraphGPT. The input of the Graph2Seq model comprises:

1. **Graph Word Prompts**  $[[\text{GW } 1], \dots, [\text{GW } k]]$ , which are identical to the word prompts discussed in Section 3.2.
2. **Property Token Sequence**  $[[\text{QED}], [\text{SA}], [\text{logP}]]$ , which is encoded from the normalized property values  $\bar{v}_{\text{QED}}$ ,  $\bar{v}_{\text{SA}}$  and  $\bar{v}_{\text{logP}}$ .
3. **Scaffold Flexible Token Sequence**  $\text{FTSeq}_{\text{Scaf}}$ , representing the sequence of the scaffold for the molecule.

For the sake of comparison, we followed Bagal et al. (2021) and trained a MolGPT model on the GuacaMol dataset (Brown et al., 2019) using QED, SA, logP, and scaffolds as conditions for 10 epochs. We compare the conditional generation ability by measuring the MAD (Mean Absolute Deviation), SD (Standard Deviation), validity and uniqueness. Table 7 presents the full results, underscoring the superior control of GraphGPT-1W-C over molecular properties.

|               | Pretrain | Metric     | QED=0.5 | QED=0.7 | QED=0.9 | SA=0.7 | SA=0.8 | SA=0.9 | logP=0.0 | logP=2.0 | logP=4.0 | Avg.         |
|---------------|----------|------------|---------|---------|---------|--------|--------|--------|----------|----------|----------|--------------|
| MolGPT        | ✗        | MAD ↓      | 0.081   | 0.082   | 0.097   | 0.024  | 0.019  | 0.013  | 0.304    | 0.239    | 0.286    | <u>0.127</u> |
|               |          | SD ↓       | 0.065   | 0.066   | 0.092   | 0.022  | 0.016  | 0.013  | 0.295    | 0.232    | 0.258    | <b>0.118</b> |
|               |          | Validity ↑ | 0.985   | 0.985   | 0.984   | 0.975  | 0.988  | 0.995  | 0.982    | 0.983    | 0.982    | <u>0.984</u> |
| GraphGPT-1W-C | ✗        | MAD ↓      | 0.041   | 0.031   | 0.077   | 0.012  | 0.028  | 0.031  | 0.103    | 0.189    | 0.201    | <u>0.079</u> |
|               |          | SD ↓       | 0.079   | 0.077   | 0.121   | 0.055  | 0.062  | 0.070  | 0.460    | 0.656    | 0.485    | <u>0.229</u> |
|               |          | Validity ↑ | 0.988   | 0.995   | 0.991   | 0.995  | 0.991  | 0.998  | 0.980    | 0.992    | 0.991    | <u>0.991</u> |
|               | ✓        | MAD ↓      | 0.032   | 0.033   | 0.051   | 0.002  | 0.009  | 0.022  | 0.017    | 0.190    | 0.268    | <b>0.069</b> |
|               |          | SD ↓       | 0.080   | 0.075   | 0.090   | 0.042  | 0.037  | 0.062  | 0.463    | 0.701    | 0.796    | <u>0.261</u> |
|               |          | Validity ↑ | 0.996   | 0.998   | 0.999   | 0.995  | 0.999  | 0.996  | 0.994    | 0.990    | 0.992    | <b>0.995</b> |

Table 7: Overall comparison between GraphGPT-1W-C and MolGPT on different properties with scaffold SMILES “c1ccccc1”. “MAD” denotes the Mean Absolute Deviation of the property value in generated molecules compared to the oracle value. “SD” denotes the Standard Deviation of the generated property.

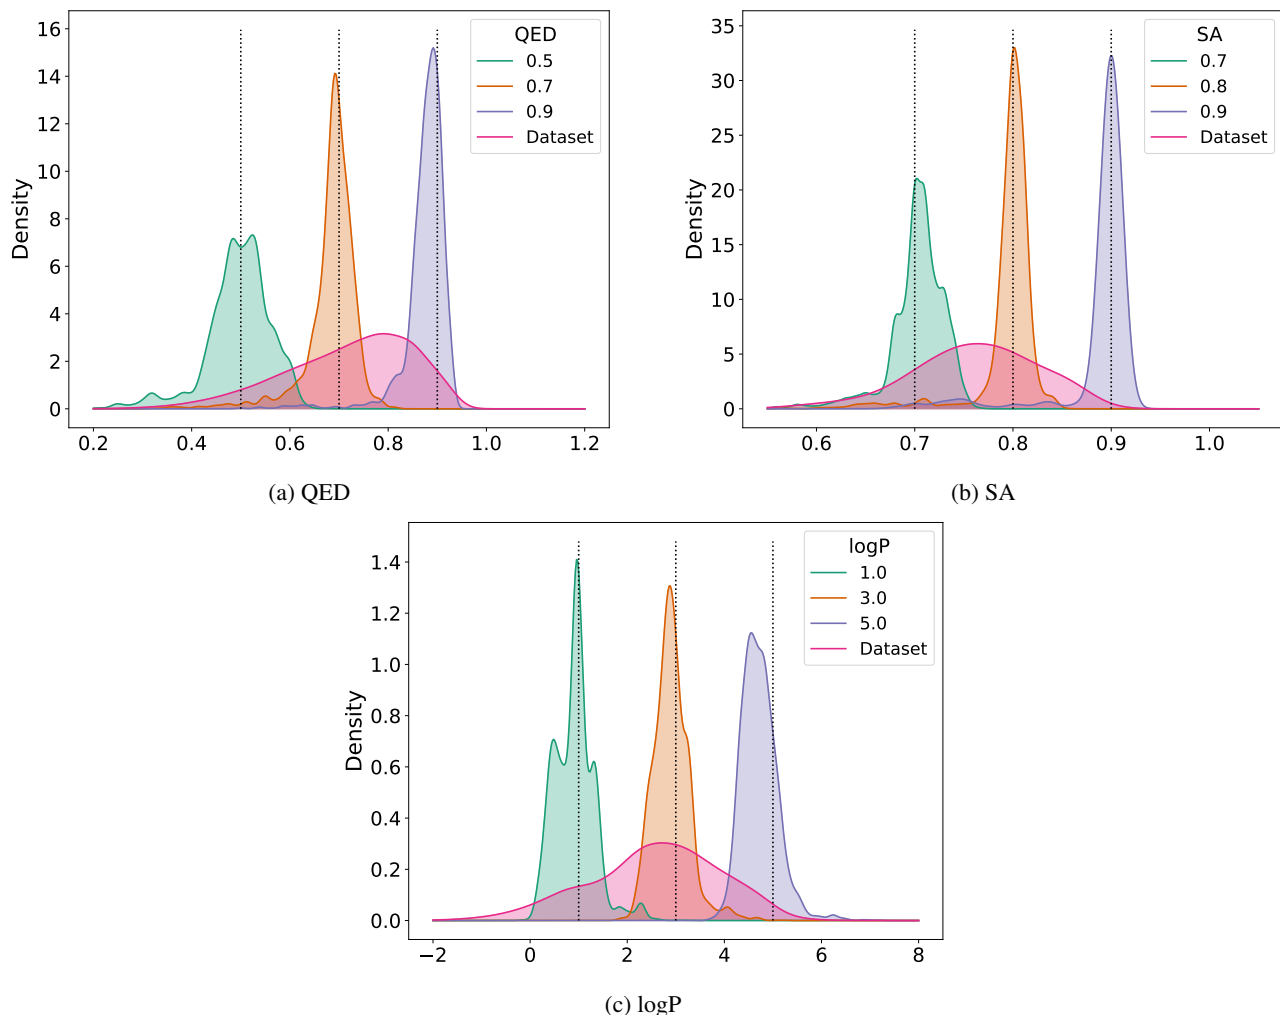

Figure 6: Property distribution of generated molecules on different conditions using GraphsGPT-1W-C.

## C. Graph Words

### C.1. Clustering

The efficacy of the Graph2Seq encoder hinges on its ability to effectively map non-Euclidean graphs into Euclidean latent features in a structured manner. To investigate this, we visualize the latent graph words space using sampled features, encoding 32,768 molecules with Graph2Seq-1W and employing HDBSCAN (?) for clustering the graph words.

Figures 7 and 8 respectively illustrate the clustering results and the molecules within each cluster. An intriguing observation emerges from these results: the Graph2Seq model exhibits a propensity to cluster molecules with similar properties (e.g., identical functional groups in clusters 0, 1, 4, 5; similar structures in clusters 2, 3, 7; or similar Halogen atoms in cluster 3) within the latent graph words space. This insight could potentially inform and inspire future research.

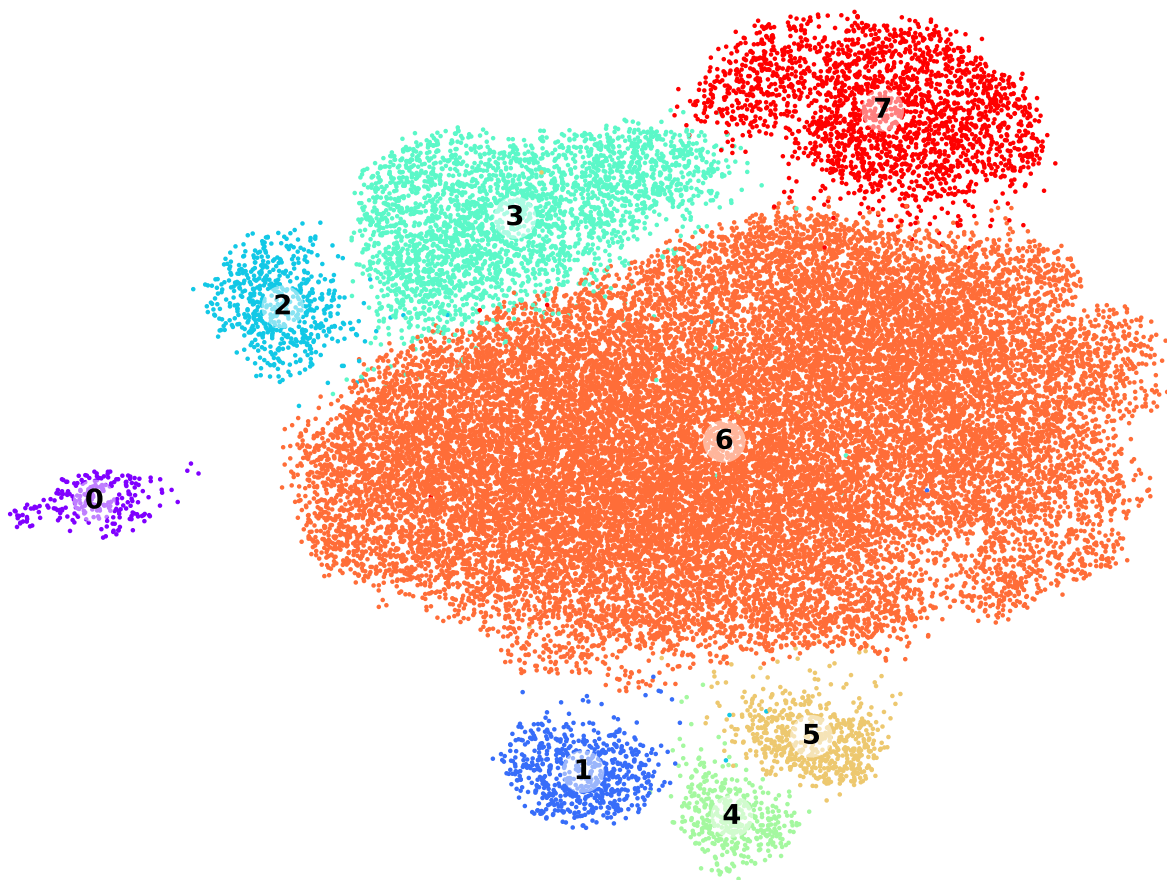

Figure 7: UMAP (McInnes et al., 2018) visualization of the clustering result on the graph words of Graph2Seq-1W.

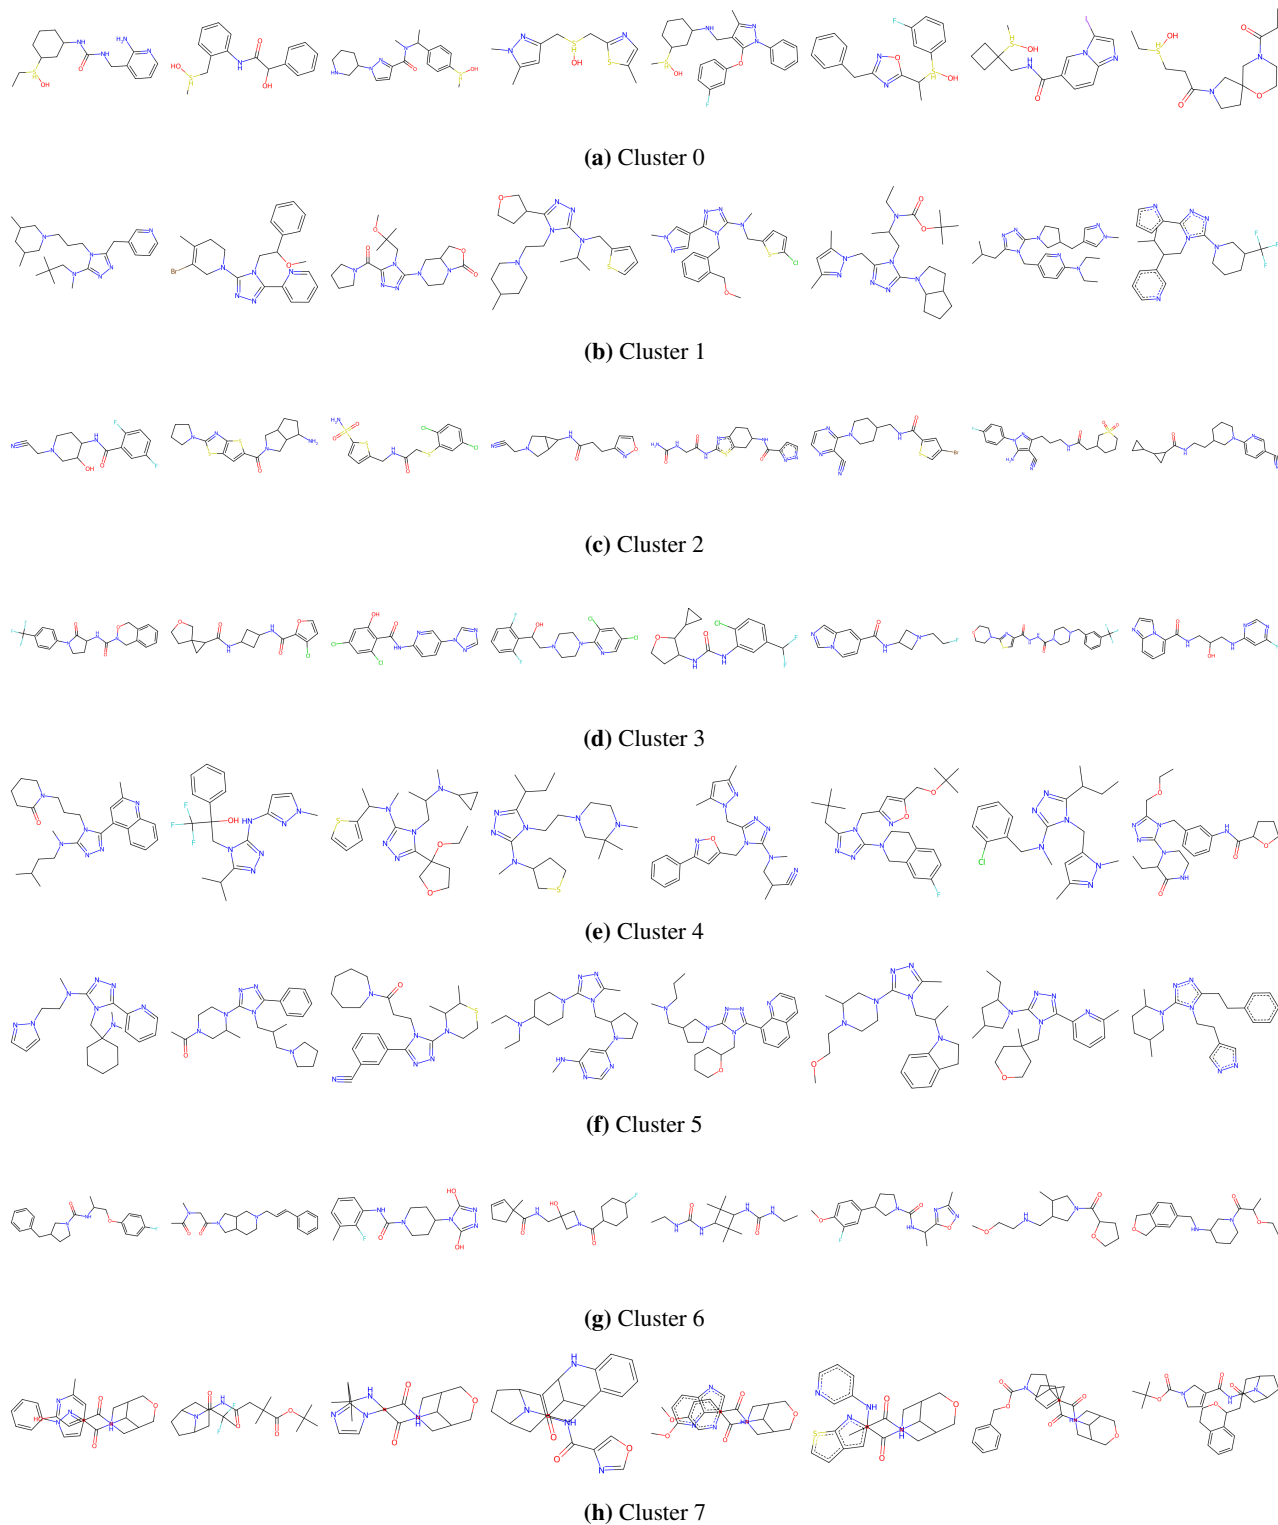

Figure 8: Visualization of the molecules in each cluster.

## C.2. Graph Translation

**Graph Interpolation** In exploit of the Euclidean representation of graphs, we explore the continuity of the latent graph words using interpolation. Consider a source molecule  $\mathcal{G}_s$  and a target molecule  $\mathcal{G}_t$ . We utilize Graph2Seq to encode them into graph words, represented as  $\mathcal{W}_s$  and  $\mathcal{W}_t$ , respectively. We then proceed to conduct a linear interpolation between these two graph words, resulting in a series of interpolated graph words:  $\mathcal{W}'_{\alpha_1}, \mathcal{W}'_{\alpha_2}, \dots, \mathcal{W}'_{\alpha_k}$ , where each interpolated graph word is computed as  $\mathcal{W}'_{\alpha_i} = (1 - \alpha_i)\mathcal{W}_s + \alpha_i\mathcal{W}_t$ . These interpolated graph words are subsequently decoded back into molecules using GraphGPT.

The interpolation results are depicted in Figure 9. We observe a smooth transition from the source to the target molecule, which demonstrates the model’s ability to capture and traverse the continuous latent space of molecular structures effectively. This capability could potentially be exploited for tasks such as molecular optimization and drug discovery.

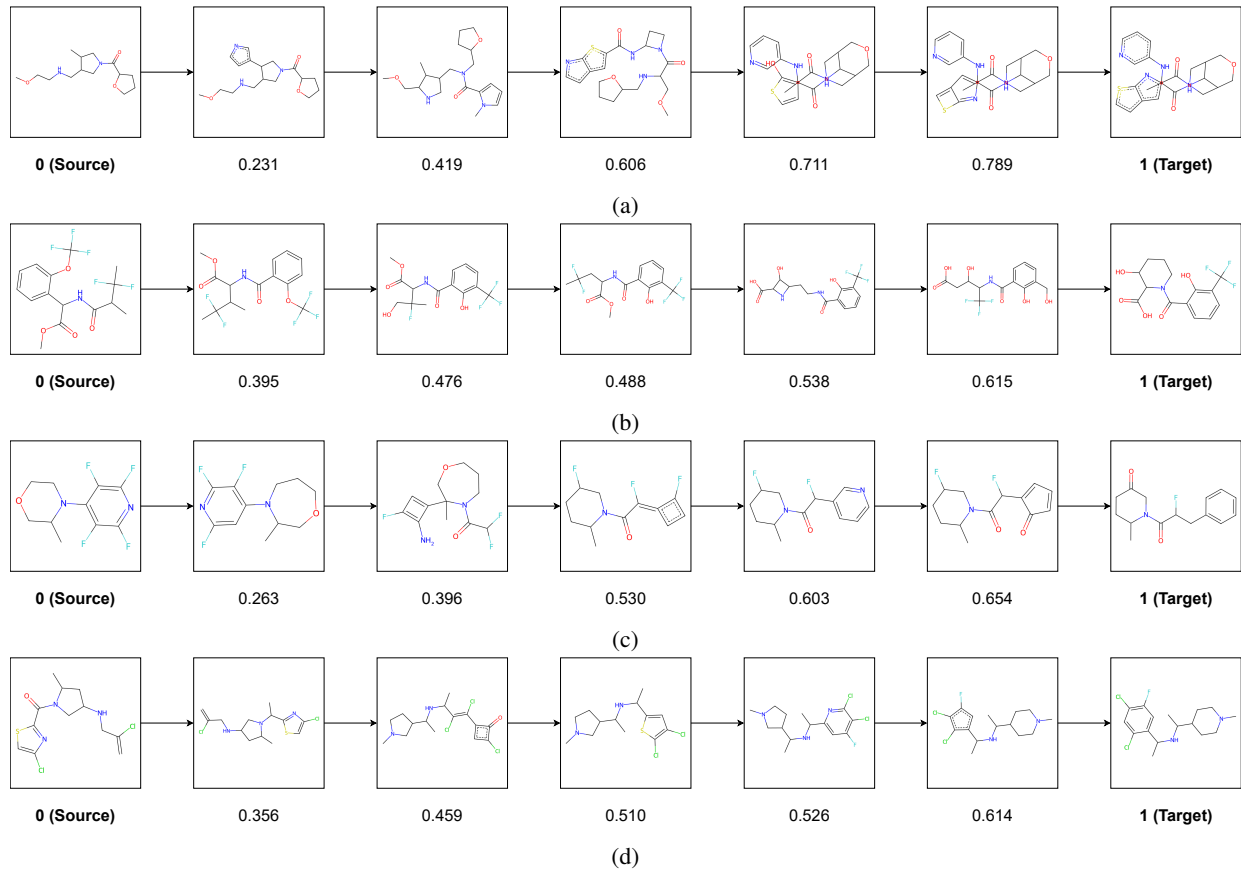

Figure 9: Graph interpolation results with different source and target molecules using GraphsGPT-1W. The numbers denote the values of  $\alpha$  for corresponding results.

**Graph Hybrid** With Graph2Seq, a graph  $\mathcal{G}$  can be transformed into a fixed-length graph word sequence  $\mathcal{W} = [w_1, \dots, w_k]$ , where each graph word is expected to encapsulate distinct semantic information. We investigate the representation of graph words by hybridizing them among different inputs.

Specifically, consider a source molecule  $\mathcal{G}_s$  and a target molecule  $\mathcal{G}_t$ , along with their graph words  $\mathcal{W}_s = [w_{s1}, \dots, w_{sk}]$  and  $\mathcal{W}_t = [w_{t1}, \dots, w_{tk}]$ . We replace a subset of source graph words with the corresponding target graph words  $w_{si} \leftarrow w_{ti}, i \in I$ , yielding the hybrid graph words  $\mathcal{W}_h = [w_{h1}, \dots, w_{hk}]$ , where:

$$w_h = \begin{cases} w_{ti}, & i \in I \\ w_{si}, & i \notin I \end{cases} \quad (15)$$

We then decode  $\mathcal{W}_h$  using GraphGPT back into the graph and observe the changes. The results are depicted in Figure 10. From these results, we observe that hybridizing specific graph words can lead to the introduction of certain features from the target molecule into the source molecule, such as the “S-OH” functional group. This suggests that graph words could potentially be used as a tool for manipulating specific features in molecular structures, which could have significant implications for molecular design and optimization tasks.

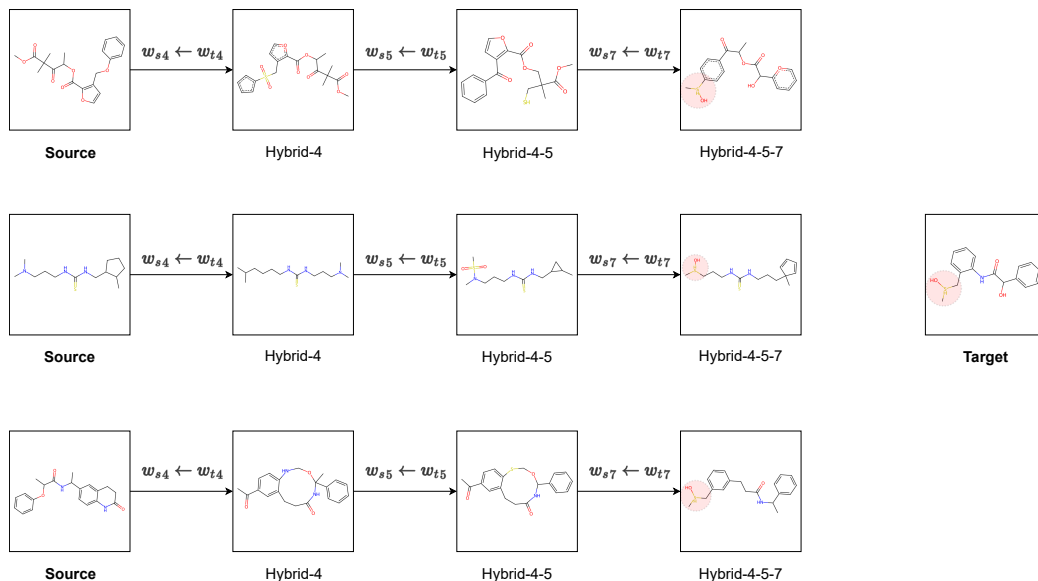

Figure 10: Hybridization results of graph words. The figure shows the changes in the source molecule after hybridizing specific graph words from the target molecule. We use GraphsGPT-8W which has 8 graph words in total.
